# Supplementary material for: Homoclinic connections with many loops near a $0^2 iw$ resonant fixed point for Hamiltonian systems
Source: arXiv:1401.1509 source file (2014-01-07)
Supplement: Supplementary file 1 [file AppendixAeng.tex]

This appendix is devoted to the statement and proof of the general Hamiltonian Normal Form Theorem \ref{ThmNF} used in Part \ref{PartieFormeNormale}. We thank G\'erard Iooss who suggested us this version and this proof of the Normal Form Theorem.

\begin{thm}[Normal form theorem]\label{ThmNF}
Let $\R^{2m}$ be endowed with the symplectic form $\Omega_m$ given by
\begin{equation}\label{EqMatrixOmegam}
\Omega_m(x,y) = \scal{J_mx}{y} \qquad \textrm{ o˘ }\qquad  J_m= \left (\begin{array}{cc}           0 & I_m \\           -I_m & 0                      \end{array}    \right).
\end{equation}
Let ${\cal U}_\Lambda$ be an open set of a Banach space $\Lambda$ such that $0\in{\cal U}_\Lambda$. Let $\Hcal_\lb$
%$$   \Hcal : {\cal U}_\Lambda\to C^k(\R^{2m};\R) :  \lb \mapsto \Hcal_\lb  $$
with $\lb\in{\cal U}_\Lambda$, be a $C^1$ one parameter family of $\C^k$ (\textit{resp. analytic and in $\An\left(\B_{\R^4}(0,\rho),\R\right)$}) Hamiltonian such that $D_x\Hcal_\lb(0)=0$. We denote by $\Hcal_{2,\lb}(x)=\frac{1}{2} D_{x,x}^2\Hcal_\lb(0).[x,x]$ the quadratic part of $\Hcal_\lb$ and by $L_0$ the linear part at $\lb=0$ of the associated hamiltonian vector field, $\ie$ $L_0x=J_m\nabla_{\hsp[-.5]x}\Hcal_{2,0}(x)$.

\vspace{1ex}

\noindent Then, for all $n$ and $k$ such that $k-1\geq n\geq 3$ (\textit{resp. for all $n\geq3$}), there exists a $\C^1$ one parameter family $\phi_{n,\lb}$ of canonical analytic mappings in $\An\left(\B_{\R^4}(0,\rho'),\R\right)$, close to identity, defined in a neighborhood of $0$ in $\Lambda$, such that in the neighborhood of $0$ in $\R^{2m}$, ${\cal H}_\lb$ satisfy
$$\begin{array}{ll}  
\Hcaltilde_{\lb}(\xtilde) = {\cal H}_\lb(\phi_{n,\lb}(\xtilde)) = \Hcal_{2,0}(\xtilde)+\Ncaltilde_{n,\lb} (\xtilde)+\Rcaltilde_{n,\lb} (\xtilde)
\end{array},$$
where  $\Ncaltilde_{n,\lb}$ is a real polynomial of degree less than $n$, and $\Rcaltilde_{n,\lb}$ is $\C^k$ (\textit{resp. belongs to $\An\left(\B_{\R^4}(0,\rho'),\R\right)$}) and 
\begin{eqnarray}
\Ncaltilde_{n,\lb}(\xtilde)&=&{\cal O}(\lb |\xtilde|^2+|\xtilde|^3), \qquad \Ncaltilde_{n,\lb}(\E^{t L_0^*} \xtilde)=\Ncaltilde_{n,\lb}(\xtilde) \ \ \mbox{pour tout } t\in\R, \nonumber\\
\Rcaltilde_{n,\lb}(\xtilde)&=&{\cal O}\left(|\xtilde|^{n+1}\right). \nonumber
\end{eqnarray}
Moreover, the coefficients of $\Ncaltilde_{n,\lb}$ are $C^{1}$ functions of $\lb$.
\end{thm}

\begin{rem}
The main consequence is that, unlike the Birkhoff Normal Form results, this theorem holds for elliptic but also non elliptic fixed points, and does not require the linear part to be semi-simple.
\end{rem}

\textbf{Proof.} We proceed in several steps.

\vspace{1ex}

{\bf Step 0. Change of coordinates.} Let us use the notations introduced in the statement of the theorem. For $n\leq k-1$ (and for all $n\in\NN$ in the analytic case) we perform the Taylor expansion of order $n$ of $\Hcal_\lb$ :
$$\Hcal_\lb(x) = \sum_{\ell=2}^n \Hcal_{\ell,\lb}(x) +{\cal O}(|x|^{n+1}),$$
where $\Hcal_{\ell,\lb}$ is a $\C^1$-family of homogeneous polynomials of degree $\ell$. Moreover, let us denote 
$$\Hcal_{2,\lb}^1(x) = \Hcal_{2,\lb}(x) -\Hcal_{2,0}(x).$$
Our aim is to construct a canonical polynomial change of coordinates $x=\phi_{n,\lb}(\xtilde)$ such that the Taylor polynomial of the new Hamiltonian is as simple as possible, $\ie$ with as few monomials as possible. We look for such a canonical transformation through a generatrix function of the form
\begin{equation}\label{EqScan} 
S_\lb(q,\ptilde)=\scal{q}{\ptilde}+S^1_{2,\lb}(q, \ptilde)+\sum_{\ell=3}^n S_{\ell,\lb}(q,\ptilde)
\end{equation}
where $x=(q,p)$, $\xtilde=(\qtilde,\ptilde)$ and where $S^1_{2,\lb}$,$S_{\ell,\lb}$ are homogeneous polynomial respectively of degree 2 and $\ell$ with $S_{2,0}^1\equiv 0$. Then (\ref{EqScan}) generates an analytic canonical transformation $x=\phi_{n,\lb}(\xtilde)$ close to identity such that 
\begin{equation}\label{ImpGen}
p=\nabla_q S_\lb(q,\ptilde), \qquad \qtilde = \nabla_{\ptilde}S_\lb(q,\ptilde).
\end{equation}
After this change of coordinates the new hamiltonian reads
$$\Hcaltilde_\lb(\qtilde,\ptilde)=\Hcal_\lb(\phi_{n,\lb}(\qtilde,\ptilde))=\sum_{\ell=2}^n\Hcaltilde_{\ell,\lb}(\qtilde,\ptilde) +{\calO}\left((|\qtilde|+|\ptilde|)^{n+1}\right).$$
and satisfies
\begin{equation}\label{EqHHtilde}   
\Hcaltilde_\lb(\nabla_{\ptilde}S_\lb(q,\ptilde),\ptilde)=\Hcal_\lb(q,\nabla_q S_\lb(q,\ptilde)).
\end{equation}

\vspace{1ex}

%%%%%%%%%%%%%%%%%%%%%%%%%%%%%%%%%%%%%%%%%%%%%%%%%%%%%%%%%%%%%%%%%%%%%%%
\textbf{Step 1 : smoothness in term of $\lb$ of the family of analytic transformations $\phi_{n,\lb}$.}

Suppose that we constructed a $\C^1$-family of generatrix functions $S_\lb$ as above. The $S_\lb$ are polynomials, so the $\phi_{n,\lb}$ are analytic functions ; let us prove that there exists $\rho$ such that $\phi_{n,\lb}$ is a $\C^1$-family of the Banach space ($\An(\B_{\R^m}(0,\rho),\R^n)$,$\NNorme{\An}{\cdot}$) of Definition \ref{DefAn}. Denoting $\phi_{n,\lb}:=(\varphi_{n,\lb},\psi_{n,\lb})$, from (\ref{ImpGen}) we get
\begin{eqnarray}
\psi_{n,\lb}(\qtilde,\ptilde)=\nabla_q S_\lb(\varphi_{n,\lb}(\qtilde,\ptilde),\ptilde) \label{GenPsi}\\
\qtilde = \nabla_{\ptilde}S_\lb(\varphi_{n,\lb}(\qtilde,\ptilde),\ptilde). \label{GenPhi}
\end{eqnarray}
The Implicit Function Theorem (IFT in the following) applied to equation (\ref{GenPhi}) allows the construction of $\varphi_{n,\lb}$. Then (\ref{GenPsi}) permits to compute $\psi_{n,\lb}$. Let us prove the smoothness of the family $\varphi_{n,\lb}$ by an appropriate use of equation (\ref{GenPhi}), proceeding in two steps :
\begin{itemize}
\item first, we fix $\lb=0$ and work in the neighborhood of $(\varphi,\qtilde,\ptilde)=(0,0,0)$. We use successively the holomorphic IFT, seeing this equation in $\CC^{2m}$ and the analytic IFT in $\R^{2m}$. Thus $\varphi$ is bounded in a ball of $\CC^{2m}$ and real-valued on the real axis. The hypotheses of the IFT are fulfilled, given that
$$D_{\varphi}\left(\nabla_{\ptilde}S_0(\varphi,\ptilde)\right)_{|(\varphi,\ptilde)=(0,0)}=I. $$
Then there exist $\rho_1$ and $\varphi_{n,0}\in\An\left(\B_{\R^{2m}}(0,\rho_1),\R^{2m}\right)$ such that 
$$\varphi_{n,0}(0,0)=0, \quad \text{and} \quad  \qtilde = \nabla_{\ptilde}S_0(\varphi_{n,0}(\qtilde,\ptilde),\ptilde) \quad \text{for all }(\qtilde,\ptilde)\in\B(0,\rho_1).$$
\item secondly, we apply the IFT to (\ref{GenPhi}) in the Banach space $\An(\B_{\R^m}(0,\rho_1),\R^n)$ in the neighborhood of $(\varphi,\lb)=(\varphi_{n,0},0)$. It is possible, up to the choice of a smaller $\rho_1$, given that
$$D_{\varphi}\left(\nabla_{\ptilde}S_\lb(\varphi,\ptilde)\right)_{|(\varphi,\ptilde)=(\varphi_{n,0},0)}=\left(D_{\qtilde}\nabla_{\ptilde}S_\lb\right)(\varphi_{n,0}(\qtilde,\ptilde),\ptilde)=I+{\cal O}((\qtilde,\ptilde)).$$
\end{itemize}
Finally, $\varphi_{n,\lb}$ is a $\C^1$-family of $\An(\B_{\R^m}(0,\rho_1),\R^n)$.

\vspace{1ex}

%%%%%%%%%%%%%%%%%%%%%%%%%%%%%%%%%%%%%%%%%%%%%%%%%%%%%%%%%%%%%%%%%%%%%%%%%%%%%%%%%%%%%%%%%%%%%%%%%%%%%%%%%%%%%%%%%%%%%%%%%%%%%%%%%%%%%%%
{\bf Step 2.1 Equation at order 2.} First, denoting 
$$\Hcaltilde_{2,\lb}^1(x) = \Hcaltilde_{2,\lb}(x) -\Hcaltilde_{2,0}(x),$$ 
our choice (\ref{EqScan}) of the form of the generatrix function ensures that $\Hcal_{2,0}=\Hcaltilde_{2,0}$. Then, identifying the powers of order 2 of $z=(q,\ptilde)$ in (\ref{EqHHtilde}) we get 
$$  \begin{array}{l}   \Hcaltilde_{2,\lb}^1(z)+\scal{\nabla_q\Hcaltilde_{2,\lb}(z)}{\nabla_{\ptilde}S^1_{2,\lb}(z)}+D^2_{qq}\Hcaltilde_{2,\lb}(z).[\nabla_{\ptilde}S^1_{2,\lb}(z),\nabla_{\ptilde} S^1_{2,\lb}(z)]\\ =   \Hcal_{2,\lb}^1(z)+\scal{\nabla_{\ptilde} \Hcal_{2,\lb}(z)}{\nabla_{q}S^1_{2,\lb}(z)}+D^2_{\ptilde\ptilde}\Hcaltilde_{2,\lb}(z).[\nabla_{q}S^1_{2,\lb}(z),\nabla_{q} S^1_{2,\lb}(z)].   \end{array}$$
Hence $\Hcaltilde_{2,\lb}^1, S_{2,\lb}^1,\Hcal_{2,\lb}^1$ are solutions of the functional equation
\begin{equation}\label{EqF2}  
\Hcaltilde_{2}^1(z)-D_{z} S_{2}^1(z).L_0z = {\cal G}_2(\Hcaltilde_{2}^1,S_{2}^1,\Hcal_{2}^1)(z)
\end{equation}
where $L_0x=J_m\nabla_{_x} \Hcal_{2,0}(x)=\bigl(\nabla_p\Hcal_{2,0}(x),-\nabla_q\Hcal_{2,0}(x)\bigr)$ and
$$\begin{array}{l} 
L_0x=J_m\nabla_{_x} \Hcal_{2,0}(x)=\bigl(\nabla_p\Hcal_{2,0}(x),-\nabla_q\Hcal_{2,0}(x)\bigr)\lba 
{\cal G}_2 (\Hcaltilde_{2}^1,S_{2}^1,\Hcal_{2}^1)(z)=  \Hcal_2^1(z)-  \scal{\nabla_q \Hcaltilde_{2}^1(z)}{\nabla_{\ptilde} S^1_{2}(z)}+\scal{\nabla_{\ptilde} \Hcal^1_{2}(z)}{\nabla_{q} S^1_{2}(z)}\lba
-D^2_{qq}(\Hcal_{2,0}+\Hcal_{2}^1)(z).[\nabla_{\ptilde}S^1_{2}(z),\nabla_{\ptilde} S^1_{2}(z)]+D^2_{\ptilde\ptilde}(\Hcaltilde_{2,0}+\Hcaltilde_{2}^1)(z).[\nabla_{q}S^1_{2}(z),\nabla_{q} S^1_{2}(z)]
\end{array}$$
 
\vspace{1ex} 
 
{\bf Step 2.2. Equation at order $\mathbf{\ell}$ with $\mathbf{3\leq\ell\leq n}$}. Identifying  the powers of order 3 of $z=(q,\ptilde)$ in  (\ref{EqHHtilde}), we get 
$$\begin{array}{l}    
\Hcaltilde_{3,\lb}(q+\nabla_{\ptilde} S_{2,\lb}^1(z),\ptilde)   +\scal{\nabla_q \Hcaltilde_{2,\lb}\Bigl(q+\nabla_{\ptilde}S^1_{2,\lb}(z),\ptilde\Bigr)}{\nabla_{\ptilde} S_{3,\lb}(z)}=\lba    \hspace{20ex}\Hcal_{3,\lb}(q,\ptilde+\nabla_{q} S_{2,\lb}^1(z))   +\scal{\nabla_q \Hcaltilde_{2,\lb}\Bigl(q,\ptilde+\nabla_{q}S^1_{2,\lb}(z)\Bigr)}{\nabla_{q} S_{3,\lb}(z)}
\end{array}$$
which reads
\begin{equation}
{\cal F}_3(\Hcaltilde_{3,\lb}, S_{3,\lb}, \lb)=0, 
\end{equation}
where ${\cal F}_3(\Hcaltilde_{3}, S_{3}, 0)= \Hcaltilde_{3}(z)-D_{z}S_{3}(z).L_0z - \Hcal_{3,0}.$

\vspace{1ex} 

Similarly, for $3\leq \ell\leq n$ we get 
\begin{equation}\label{EqFl}
{\cal F}_\ell(\Hcaltilde_{\ell,\lb}, S_{\ell,\lb}, \lb)=0, 
\end{equation}
with
$${\cal F}_\ell(\Hcaltilde_{\ell}, S_{\ell}, 0)= \Hcaltilde_{\ell}(z)-D_{z}S_{\ell}(z).L_0z - \Hcal_{\ell,0}+R_\ell(z)$$
where ${\cal F}_\ell$ only depends of $\Hcaltilde^1_{2,\lb},S^1_{2,\lb}, \Hcal^1_{2,\lb}$, $\Hcaltilde_{j\lb}, S_{j\lb},\Hcal_{j\lb}$ with $3\leq j\leq \ell$ and where $R_\ell$ only depends of $\Hcaltilde_{j,0},S_{j,0},\Hcal_{j,0}$ for$3\leq j\leq \ell-1$, ($R_3=0$).

\vspace{1ex}

So (\ref{EqF2}), \mbox{(\ref{EqFl})$_\ell$}, $3\leq \ell\leq n $, form a hierarchy of equations of unknown $\Hcaltilde^1_{2,\lb},S^1_{2,\lb}, \Hcaltilde_{\ell,\lb}, S_{\ell,\lb}$ with $3\leq \ell\leq n$ that we will solve by induction with the Implicit Function Theorem.

\vspace{1ex}

{\bf Step 3. Study of the homological operator.} Observe that the unperturbed linear part of all these equations is given by
$${\cal L} : E_\ell\times E_\ell \to E_\ell  : (\Hcaltilde, S)\to\Hcaltilde-{\cal A} S$$
where $E_\ell$ is the space of the real-valued homogeneous polynomials of degree $\ell$ and where ${\cal A}$ is the homological operator given by
$$({\cal A}S)(z) =D_{z}S(z).L_0z.$$
{\it We look for $F_\ell$ and $G_\ell$ two subspaces of $E_\ell$ such that ${\cal L} : F_\ell\times G_\ell \to E_\ell$ is invertible. Observe that $F_\ell$ is the space where we look for the nornal form monomials of degree $\ell$. So, our aim is to choose $F_\ell$ as "small" as possible and in particular we would like to have $F_\ell=\{0\}$ when it is possible.}

\vspace{1ex}

On one hand, {\bf when ${\cal A}$ is invertible} from $E_\ell$ onto $E_\ell$, then ${\cal L}$ is invertible from $\{0\}\times E_\ell\to E_\ell$. In this case we can choose $F_\ell=\{0\}$ and $G_\ell=E_\ell$. So, in this case we chose $\Hcaltilde_{\ell,\lb}=0$ and solve \mbox{(\ref{EqFl})$_\ell$} with the implicit function theorem to get $S_{\ell,\lb}$ as a $C^1$ function of $\lb$. So when ${\cal A}$ is invertible from $E_\ell$ onto $E_\ell$, all the \mbox{$\ell-$th}order term of the Hamiltonian are removed  by the normalization procedure.

On the other hand, {\bf when ${\cal A}$ is not invertible}, $F_\ell$ must be chosen as a supplementary space  of the range ${\rm Im} {\cal A}$ of ${\cal A}$ and $G_\ell$ must be chosen as a supplementary space of $\ker {\cal A}$, $\ie$
$$   E_\ell=F_\ell\oplus {\rm Im}_{_{E_\ell}} {\cal A}, \qquad E_\ell=G_\ell\oplus\ker_{_{E_\ell}} {\cal A},$$ 
so that ${\cal L}:F_\ell\times G_\ell \to E_\ell$ is invertible. In this case, neither $\Hcaltilde_{\ell,\lb}$ nor $S_{\ell,\lb}$ are unique. They both depend of the choice of $F_\ell$ and $G_\ell$. A natural way to choose these two subspaces is to endow $E_\ell$ with an inner product and to choose 
$$ F_\ell= ({\rm Im}_{_{E_\ell}} {\cal A})^\bot, \qquad G_\ell=(\ker_{_{E_\ell}} {\cal A})^\bot.$$
In what follows we define an appropriate inner product such that $F_\ell:={\rm Im} {\cal A})^\bot=\ker{\cal A^*}$ is given by
$$  F_\ell = \{ S\in E_\ell / \ S(e^{tL_0^*}z)=S(z) \ \mbox{ forall } t\in \R, z\in \R^m\}.$$
For that purpose, let us define, for any pairs of polynomials $S,S':\R^{2m}\to \R$lying in$\in E_\ell$ the inner product given  by
$$  \scal{S}{S'}_\ell= S(\partial_{z}) S'(z)|_{z=0}.$$
Endowed with this inner product $E_\ell$ is a finite dimensional Hilbert space. Observe that for any integers $\alpha_1,\cdots, \alpha_{2m}$ and $\beta_1,\cdots, \beta_{2m}$
$$\scal{z_1^{\alpha_1}\cdot \! \dots \! \cdot z_{2m}^{\alpha_{2m}}}{z_1^{\beta_1}\cdot \! \dots \! \cdot z_{2m}^{\beta_{2m}}}_\ell=\alpha_1!\cdots\alpha_{2m}!\ \delta_{\alpha_1,\beta_1}\cdots\delta_{\alpha_{2m},\beta_{2m}}$$
where $\delta_{\alpha_j,\beta_j} = 1$ if $\alpha_j=\beta_j$ and $0$ otherwise. Moreover, for any invertible linear operator on $\R^{2m}$, considering the change of coordinates $x=T^*y$ (for which $\partial_y=T\partial_x$ and observing that $x=0\Leftrightarrow y=0$), we get
$$  \scal{S\circ T}{S'}_\ell=\scal{S}{S'\circ T^*}_\ell.$$
Hence for every $t\in\R$ we have $\scal{S\circ \E^{tL_0}}{S'}_\ell=\scal{S}{S'\circ e^{tL_0^0*}}_\ell $ and differentiating this identity with respect to $t$ we finally get for $t=0$ that
$$\scal{{\cal A}S}{S'}=  \scal{D_{z}S(z).L_0z}{S'}=\scal{S}{D_{z}S(z).L_0^*z}=   \scal{S}{{\cal A}^*S'}.$$
This ensures that the adjoint ${\cal A}^*:E_\ell \to E_\ell$ of the homological operator ${\cal A}$ is given by 
$$({\cal A}^*S)(z)= D_{z}S(z).L_0^*z$$ 
and that 
\begin{equation}\label{EqKerAstar}  
\ker_{_{E_\ell}} {\cal A}^*=\{ S\in E_\ell / \ S(e^{tL_0^*}z)=S(z) \ \mbox{for all } t\in \R, z\in \R^m\}. 
\end{equation} 
Finally, let us chose as claimed above
 $$F_\ell:=\ker_{_{E_\ell}} {\cal A}^*=({\rm Im}_{_{E_\ell}} {\cal A})^\bot, \quad G_\ell=(\ker_{_{E_\ell}}{\cal A})^\bot.$$
Denote by $\pi_\ell$ the orthogonal projection onto $\ker_{_{E_\ell}} {\cal A}^*$. Then,  ${\cal L} :  (\Hcaltilde, S)\mapsto \Hcaltilde-{\cal A} S$ is an isomorphism from $F_\ell\times G_\ell$ onto $E_\ell$ since, for any ${\cal G}\in E_\ell$,
$${\cal L}(\Hcaltilde,S)={\cal G}\Leftrightarrow  \Hcaltilde-{\cal A} S={\cal G}\Leftrightarrow  \left \lbrace\begin{array}{rl}\Hcaltilde & = \pi_\ell {\cal G}\\-{\cal A} S & = (Id-\pi_\ell) {\cal G}\end{array}\right.$$
where ${\cal A}$ is an isomorphism from $G_\ell=(\ker_{_{E_\ell}} {\cal A} )^\bot$ onto $(Id-\pi_\ell)E_\ell = {\rm Im}_{_{E_\ell}} {\cal A}$.

\vspace{1ex}

{\bf \noindent Step 4.1. Study of the equation of order 2.} The functional equation (\ref{EqF2}) reads 
\begin{equation}\label{EqLG2}   
{\cal L}(\Hcaltilde_2^1,S_2^1)= {\cal G}_2(\Hcaltilde_{2}^1,S_{2}^1,\Hcal_{2}^1)
\end{equation}
where ${\cal G}_2$ is an analytic function from $F_2\times G_2 \times E_2$ to $E_2$ satisfying 
$${\cal G}_2(0,0,0)=0, \qquad \sNNorme{E_2}{{\cal G}_2(\Hcaltilde_{2}^1,S_{2}^1,0)}\leq c \left(\sNNorme{E_2}{\Hcaltilde_{2}^1}+\sNNorme{E_2}{S_{2}^1}\right)^2,$$
where $F_2:=\ker_{_{E_2}} {\cal A}^*$ and  $G_2:=(\ker_{_{E_2}} {\cal A})^\bot$. Hence the Implicit Function Theorem ensures that for $\Hcaltilde_{2}^1,S_{2}^1,\Hcal_2^1$ sufficiently small, (\ref{EqLG2}) has a unique solution of the form
$$(\Hcaltilde_2^1,S_2^1) = \psi_2(\Hcal_2^1)$$
where $\psi_2 : E_2 \to F_2 \times G_2$ is analytic and satisfies $\psi_2(0)=0$. Finally, since $\Hcal_{2,\lb}^1$ is a $C^{1}$ function of $\lb$ vanishing for $\lb=0$, we get that for $\Norme{\Lambda}{\lb}<\delta_2$ with $\delta_2>0$ sufficiently small, $(\Hcaltilde_{2,\lb}^1,S_{2,\lb}^1) = \psi_2(\Hcal_{2,\lb}^1)$ are $C^{1}$ functions of $\lb$ and that $\Hcaltilde_{2,\lb}^1$ lies in $F_2=\ker_{_{E_2}}{\cal A}^*$ given by (\ref{EqKerAstar}).

\vspace{1ex}

{\bf \noindent Step 4.2. Study of the equation of order $n\geq 3$.} We start with the equation of order 3 given by \mbox{(\ref{EqFl})$_3$}. Let us denote $F_3 := \ker_{_{E_3}} {\cal A}^*$ and $G_3=(\ker_{_{E_3}} {\cal A})^\bot$ . Since $\Hcaltilde_{2,\lb}^1,S_{2,\lb}^1$ and $\Hcal_{3,\lb}$ are $C^{1}$ functions of $\lb$, the function \mbox{${\cal F}_3 : F_3\times G_3\times D_\Lambda(0,\delta_2)\to E_3$} is of class $C^{1}$ where $D_\Lambda(0,\delta)=\{\lb\in\Lambda,$ $\Norme{\Lambda}{\lb}<\delta\}$ and satisfies 
$${\cal F}_3(\Hcaltilde_{3}, S_{3}, 0)= {\cal L}(\Hcaltilde_3,S_3) -\Hcal_{3,0}.$$
Then the Implicit Function Theorem applied at the point $(\Hcaltilde_{3,0},S_{3,0},0)$ where $(\Hcaltilde_{3,0},S_{3,0})={\cal L}^{-1}(\Hcal_{3,0})$, ensures that for $\Norme{\Lambda}{\lb}<\delta_3$ with $\delta_3>0$ sufficiently small, $\Hcaltilde_{3,\lb},S_{3,\lb}$ are $C^{1}$ function of $\lb$ and that $\Hcaltilde_{3,\lb}$ lies in $F_3=\ker_{_{E_3}}{\cal A}^*$ given by (\ref{EqKerAstar}).

\vspace{1ex}

Then, proceeding by induction and solving as above at each step equation \mbox{(\ref{EqFl})$_\ell$} with the Implicit Function Theorem, we get that for $3\leq \ell\leq n$, and for $\Norme{\lb}{\Lambda}<\delta_\ell$ with $\delta_\ell>0$ sufficiently small, $\Hcaltilde_{\ell,\lb},S_{\ell,\lb}$ are $C^{1}$ functions of $\lb$ and that $\Hcaltilde_{\ell,\lb}$ lies in $F_\ell=\ker_{_{E_\ell}}{\cal A}^*$ given by (\ref{EqKerAstar}). 
\cqfd
